# Supplementary material for: Optimal Transport for Parameter Identification of Chaotic Dynamics via Invariant Measures
Source: arXiv:2104.15138 source file (2022-04-11)
Supplement: Supplementary file 1 [file ex_supplement.tex]

% SIAM Supplemental File Template
\documentclass[review,supplement,onefignum,onetabnum]{siamart190516}

%%% Local Variables: 
%%% mode:latex
%%% TeX-master: "ex_article"
%%% End: 

\externaldocument{outline}

% Optional PDF information
\ifpdf
\hypersetup{
  pdftitle={OT for Parameter Identification},
  pdfauthor={\TheAuthors}
}
\fi

\headers{OT for Parameter Identification}{\TheAuthors}

\begin{document}

\maketitle

\bibliographystyle{siamplain}
\bibliography{lorenz}

\end{document}
